# Supplementary material for: Questionnaires to PDEs: From Disorganized Data to Emergent Generative Dynamic Models
Source: arXiv:2204.11961 source file (2022-04-25)
Supplement: Supplementary file 1 [file extra_SI.tex]

\section{Dimensionality of the spatial embedding}\label{app:2D}

After subsampling and removing uninteresting pixels (Fig. \ref{fig:video_subsample}), our preprocessed data consisted of 1000 videos, with time series at 113 pixels, for 61 time units. We then ran the tree questionnaire code to get an embedding for each axis.

\begin{figure*}
    \includegraphics[width=8.9cm]{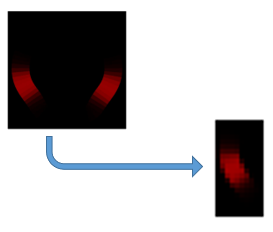}
    \caption{\label{fig:video_subsample} Example of subsampling and cropping a video frame.}
\end{figure*}

Here we show the embedding of the 113 pixels that we took trajectories from (Fig.\ref{fig:spatial_embed}). The results here are slightly counter-intuitive at first glance. The pixels have an inherent two-dimensional organization, but the algorithm only uncovers one independent embedding coordinate. This is largely because the underlying cell system is one-dimensional (i.e., a segment of a ring of cells). Another possible cause of dimensionality would be pixels that cover multiple cells, especially at the boundary of the embryo. However, in this case the variation in the chemical concentration trajectory for those pixels is too small for the algorithm to pick up, especially given the relatively low number of pixels sampled.

%the data are really discrete boxes
%this observation has 2d structure
%but we don't find it

\begin{figure*}
    \includegraphics[width=8.9cm]{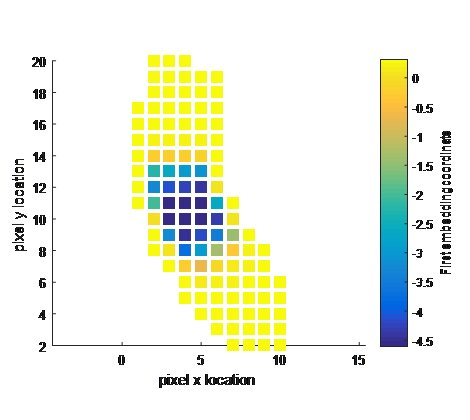}
    \caption{\label{fig:spatial_embed} Spatial embedding: 1 main embedding coordinate.}
\end{figure*}

%\section{Neural Net representation {\em of the solution} as a function of emergent coordinates}
\label{app:NN_sol}
%\comment{It seems a bit grandiose to call this a "model" since we only learned the solution.}
Before learning a dynamic PDE model capable of generating the data, we also 
trained a neural net to simply learn {\em the pixel intensity data}
for a given point in our parameter, space, and time embeddings. 
%Since the two-dimensional time embedding is visually recognizable as a one-dimensional path, we approximated an arc length $\omega$ in the embedding space using linear interpolation from point to point. 
Thus, the neural net had 4 inputs: $\phi_1$ and $\phi_2$ (the two parameter embedding coordinates), $\psi_1$ (the pixel embedding coordinate), and $\omega$ (our proxy for time). It would also have been reasonable to use both $\tau_1$ and $\tau_2$, or to assume true timestamps were known and use those.

The network had eight hidden layers of width twelve with $\tanh$ activation. That is, the network can be recursively defined as
\begin{equation}
\begin{array}{rcl}
     \vec{y} &=& \vec{h}_M \cdot \mat{W}_M + \vec{b}_{M} \\
     \vec{h}_{k+1} &=& \tanh(\vec{h}_k \cdot \mat{W}_k + \vec{b}_k) \\
     \vec{h}_0 = &=& [\phi_1, \phi_2, \psi_1, \omega] \\
     k &=& 0, 1, ..., M \\
     M &=& 12,\\
\end{array}
\end{equation}
where the 1,165 learnable parameters comprise the weight matrices $\mat{W}_0,\ldots,\mat{W}_M$ and the bias vectors $\vec{b}_0,\ldots,\vec{b}_M$.

%\comment{
%    If you want to talk about learning continuous-time systems from this data, you could cite [1] for ODEs, and then [2] for the PDE-specific additions.
%    \begin{enumerate}
%        \item Rico-Martínez, Ramiro, Katharina Krischer, Ioannis G Kevrekidis, M. C. Kube, and J. L. Hudson. “Discrete- vs Continuous-Time Nonlinear Signal Processing of Cu Electrodissolution Data.” Chemical Engineering Communications 118, no. 1 (1992): 25–48. https://doi.org/10.1080/00986449208936084.
%       \item González-García, R., Ramiro Rico-Martínez, and Ioannis G Kevrekidis. “Identification of Distributed Parameter Systems: A Neural Net Based Approach.” Computers \& Chemical Engineering 22, no. 98 (March 1998): S965–68. https://doi.org/10.1016/S0098-1354(98)00191-4.
%\end{enumerate}
%}

\begin{figure*}
    \includegraphics[width=17.8cm]{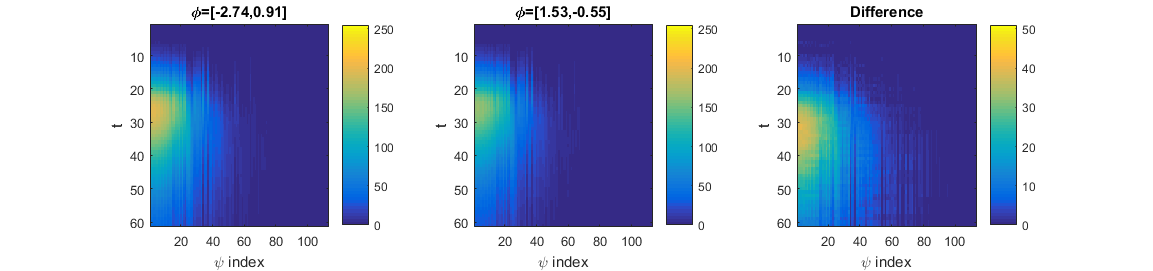}
    \caption{\label{fig:test_diff} Comparison of data from two test parameter settings.}
\end{figure*}

\begin{figure*}
    \includegraphics[width=17.8cm]{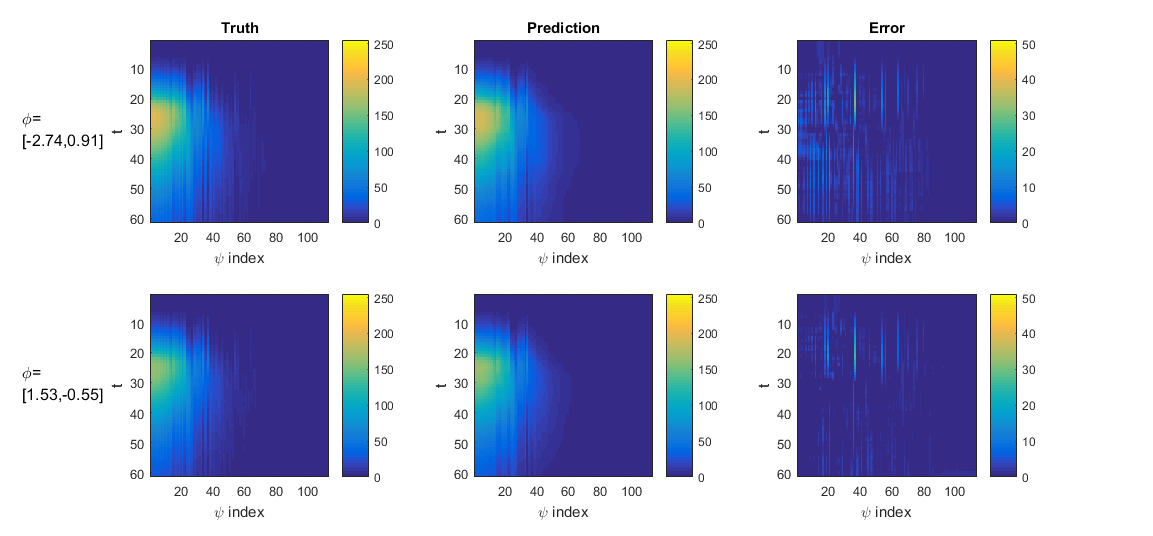}
    \caption{\label{fig:test} Reconstruction of data from two test parameter settings.}
\end{figure*}
