# Supplementary material for: Questionnaires to PDEs: From Disorganized Data to Emergent Generative Dynamic Models
Source: arXiv:2204.11961 source file (2022-04-25)
Supplement: Supplementary file 2 [file SI.tex]

The resulting data is shown in Fig.~\ref{fig:learn_data}(right).
Note that we repeat this data sampling procedure for each of the 1000 parameter settings.\\
\begin{figure*}
    \includegraphics[width=\textwidth]{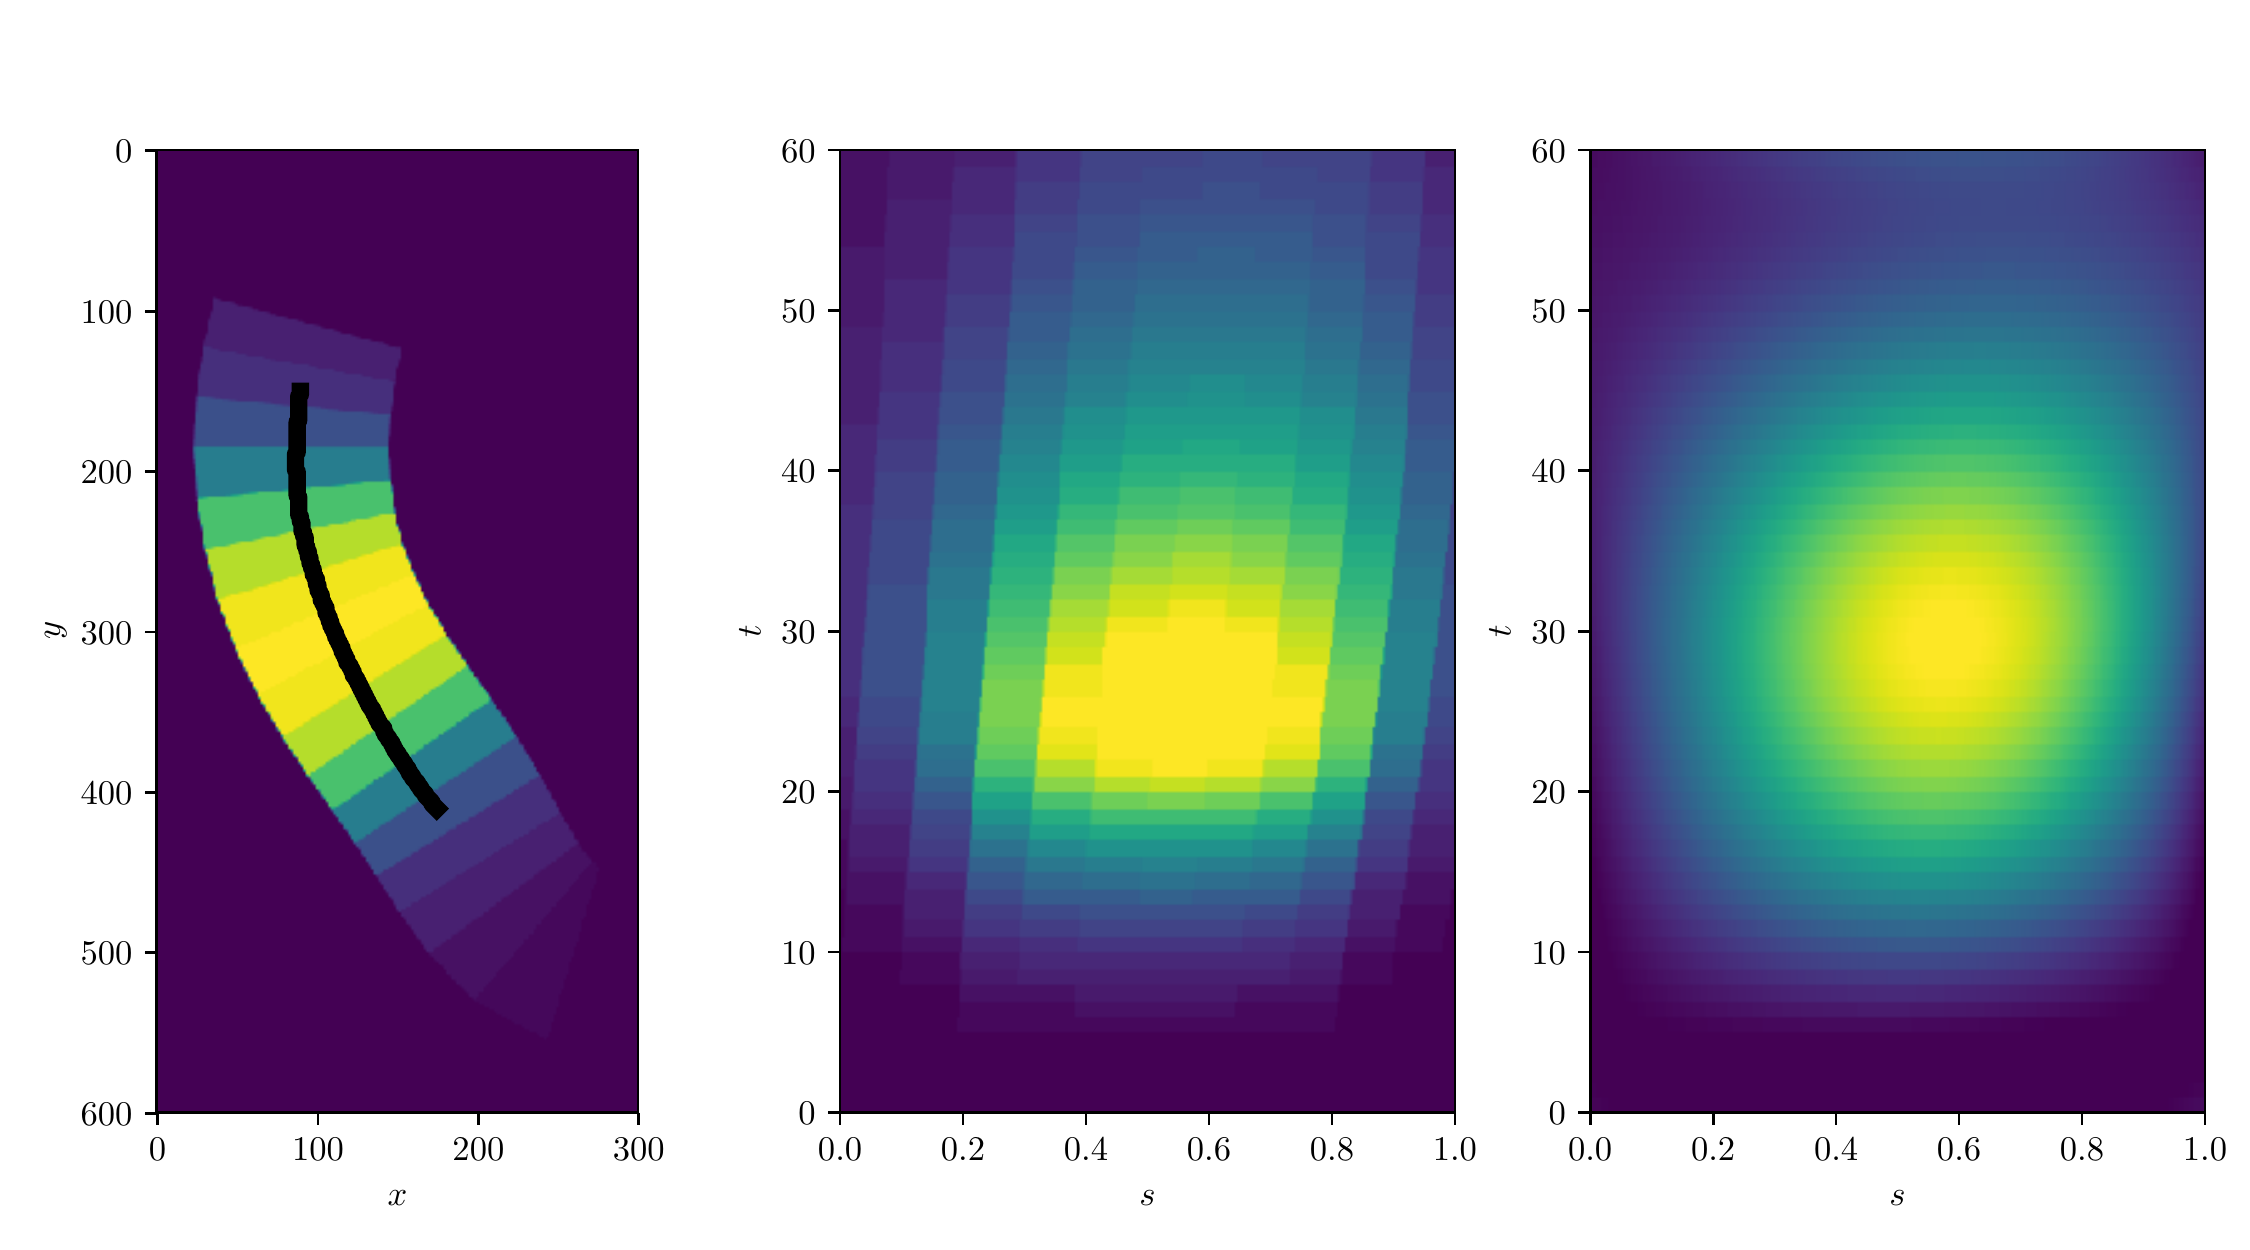}
    \caption{Left: Snapshot of a concentration profile for one parameter setting at $t=30$. The black curve indicates the one-dimensional region at which data is sample.
      Middle: Data recorded at the black curve shown on the left as a function of the
      arc length $s$ of that curve.
      Right: Data, as shown in the middle, but fitted using a bivariate spline approximation.
    The color coding in all figures encodes the concentration $c$.}
    \label{fig:learn_data}
\end{figure*}

\begin{figure*}
    \includegraphics[width=17.8cm]{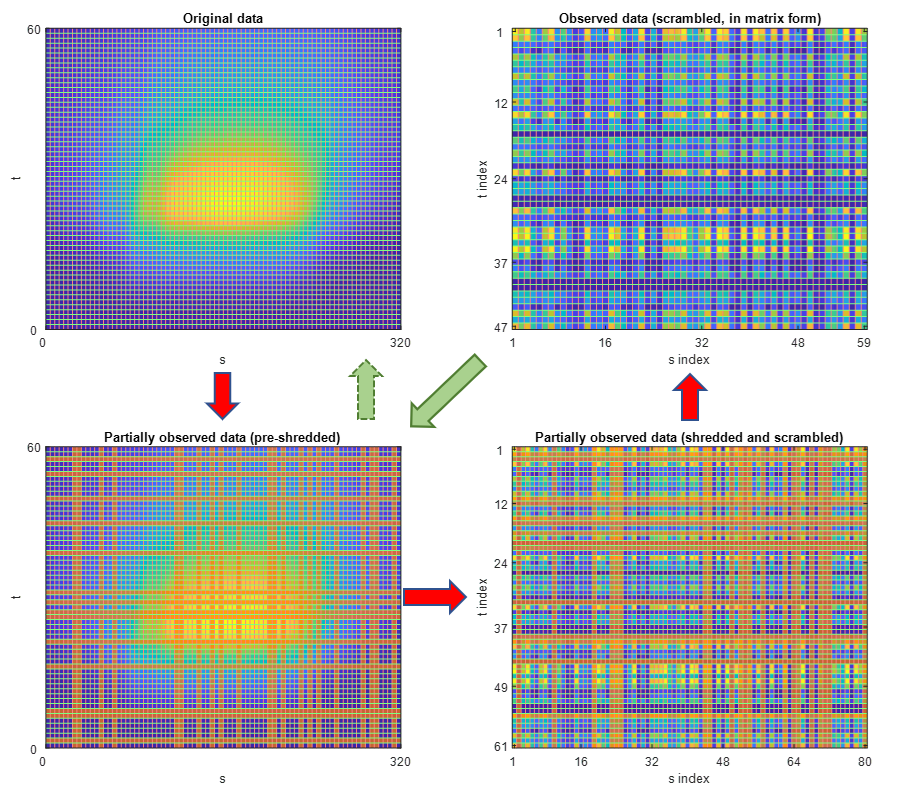}
    \caption{\label{fig:embryo_scramble} Caricature of data shredding and scrambling. \textit{(Top Left)} The full data field. Each grid box represents a potentially multi-dimensional data collection point. \textit{(Bottom Left)} We only have access to the field at independent random samplings of $x$ and $y$. We do not have access to the orange shaded grid boxes. \textit{(Bottom Right)} By scrambling the indices $x$ and $y$, we "shred" the data. However, the grid boxes in a particular column same column remain together, as do the grid boxes in a particular row. \textit{(Top right)} After we have removed empty rows and columns, this data is the input to our algorithm. \textit{Solid green arrow} We will use diffusion maps with the questionnaire metric to unscramble our data, both reordering them and placing them correctly in space (more accurately, in new space embedding coordinates that are one to one with physical space). \textit{Dashed green arrow} Various interpolation methods can be used to fill in the missing areas of the field.}
\end{figure*}

\begin{figure*}
    \includegraphics[width=\textwidth]{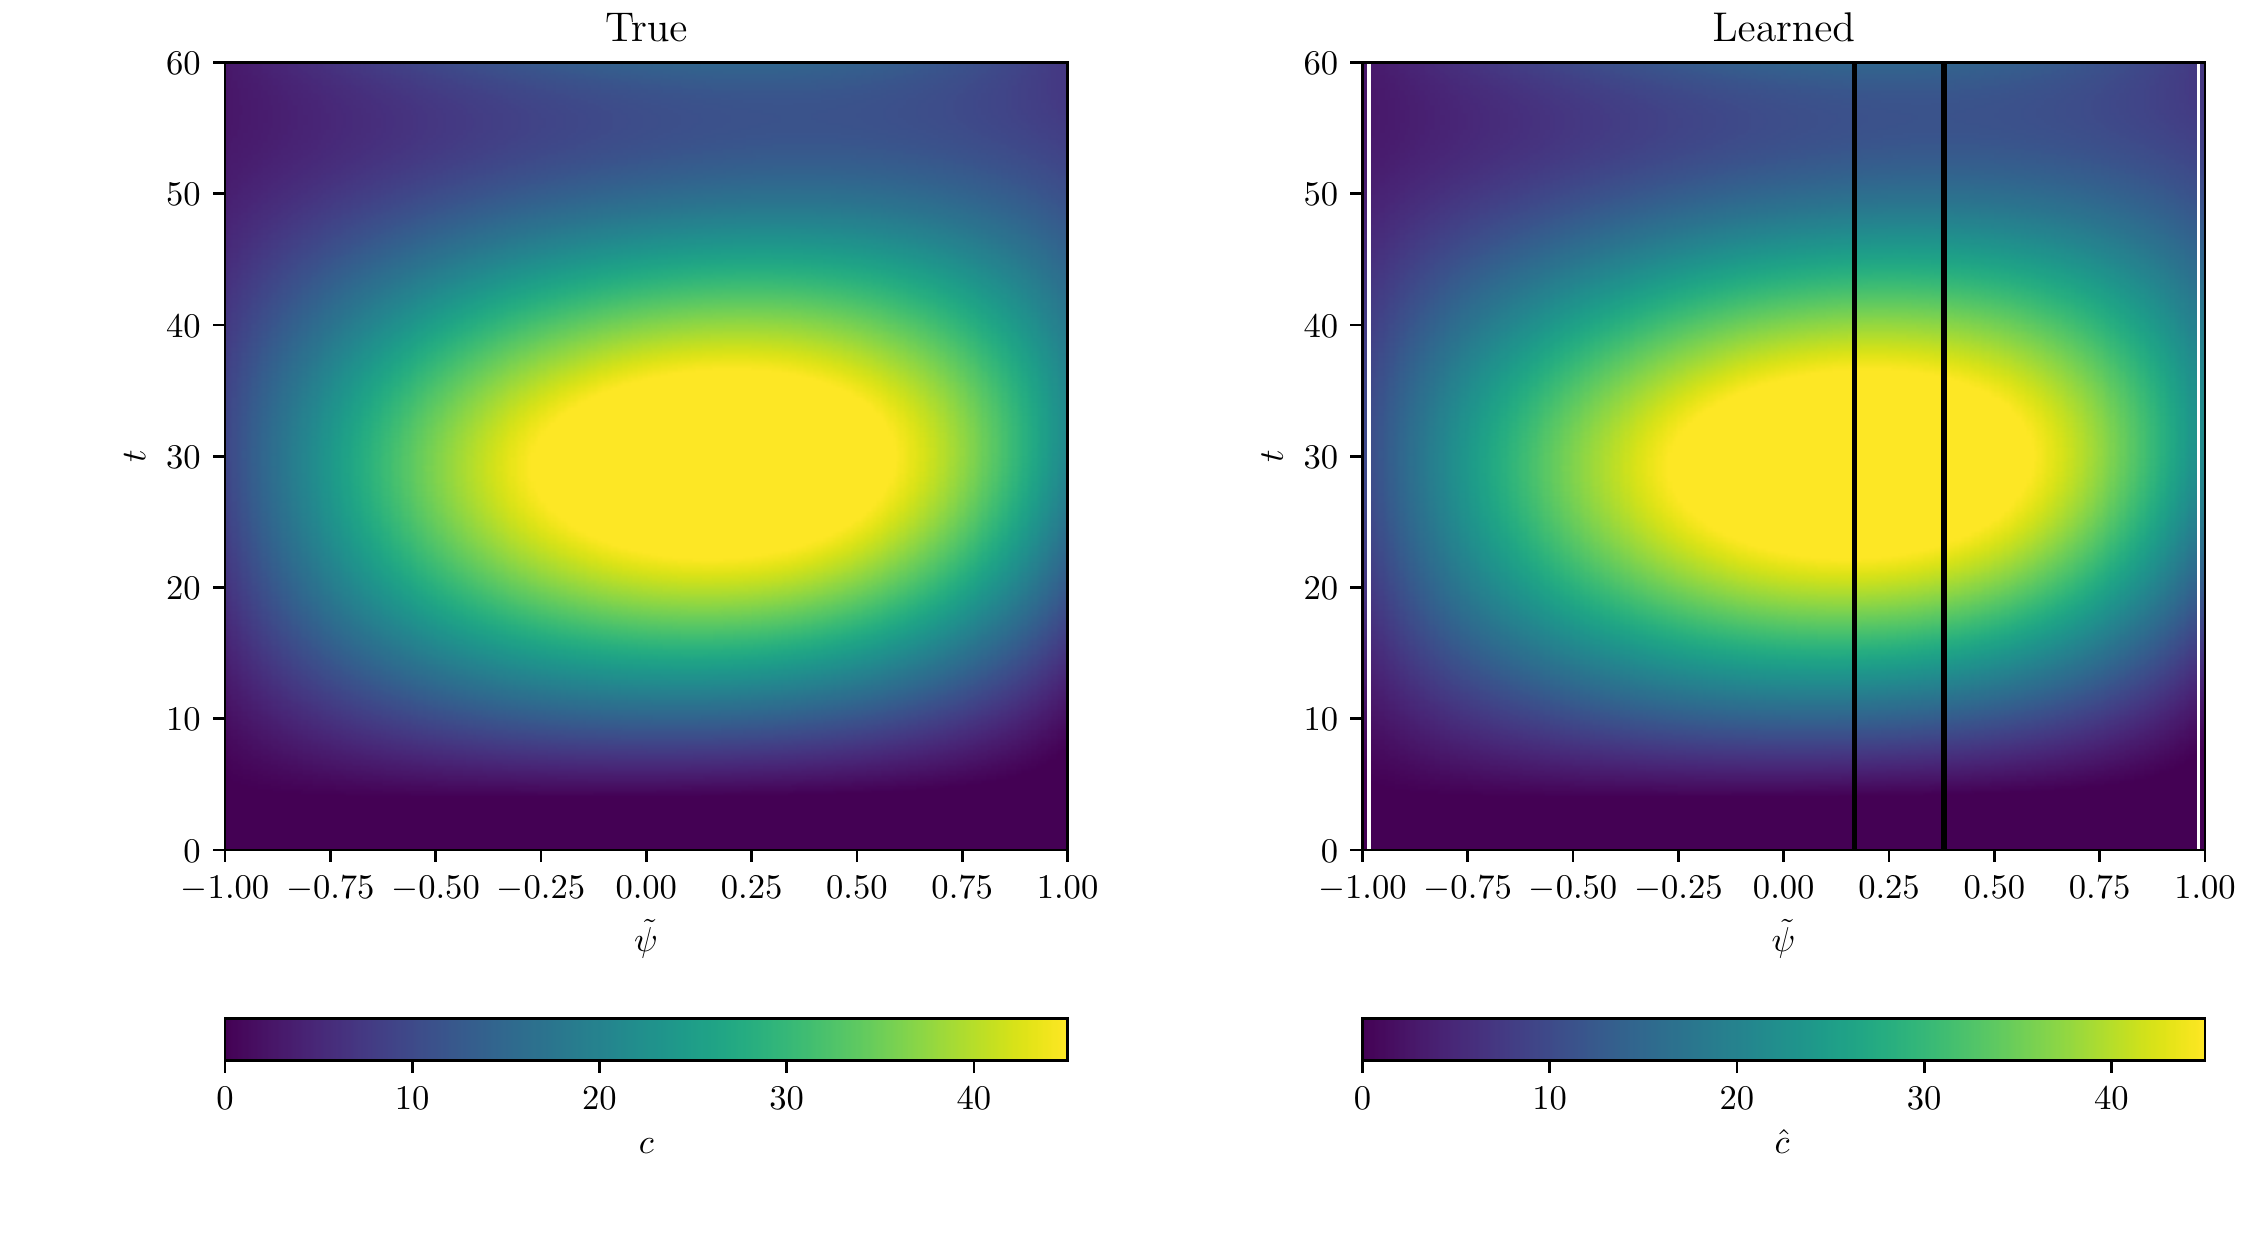}
    \caption{Left: True data as shown in Fig.~\ref{fig:learn_space}(right). Right: Data obtained by integrating the initial snapshot of the data shown on the left, but using the learned model $f$. Thereby, boundaries are provided, as indicated by the white vertical lines. In addition, the corridor around the source term is provided, as indicated by the black vertical lines.}
    \label{fig:learn_results}
\end{figure*}

\begin{figure*}
    \includegraphics[width=\textwidth]{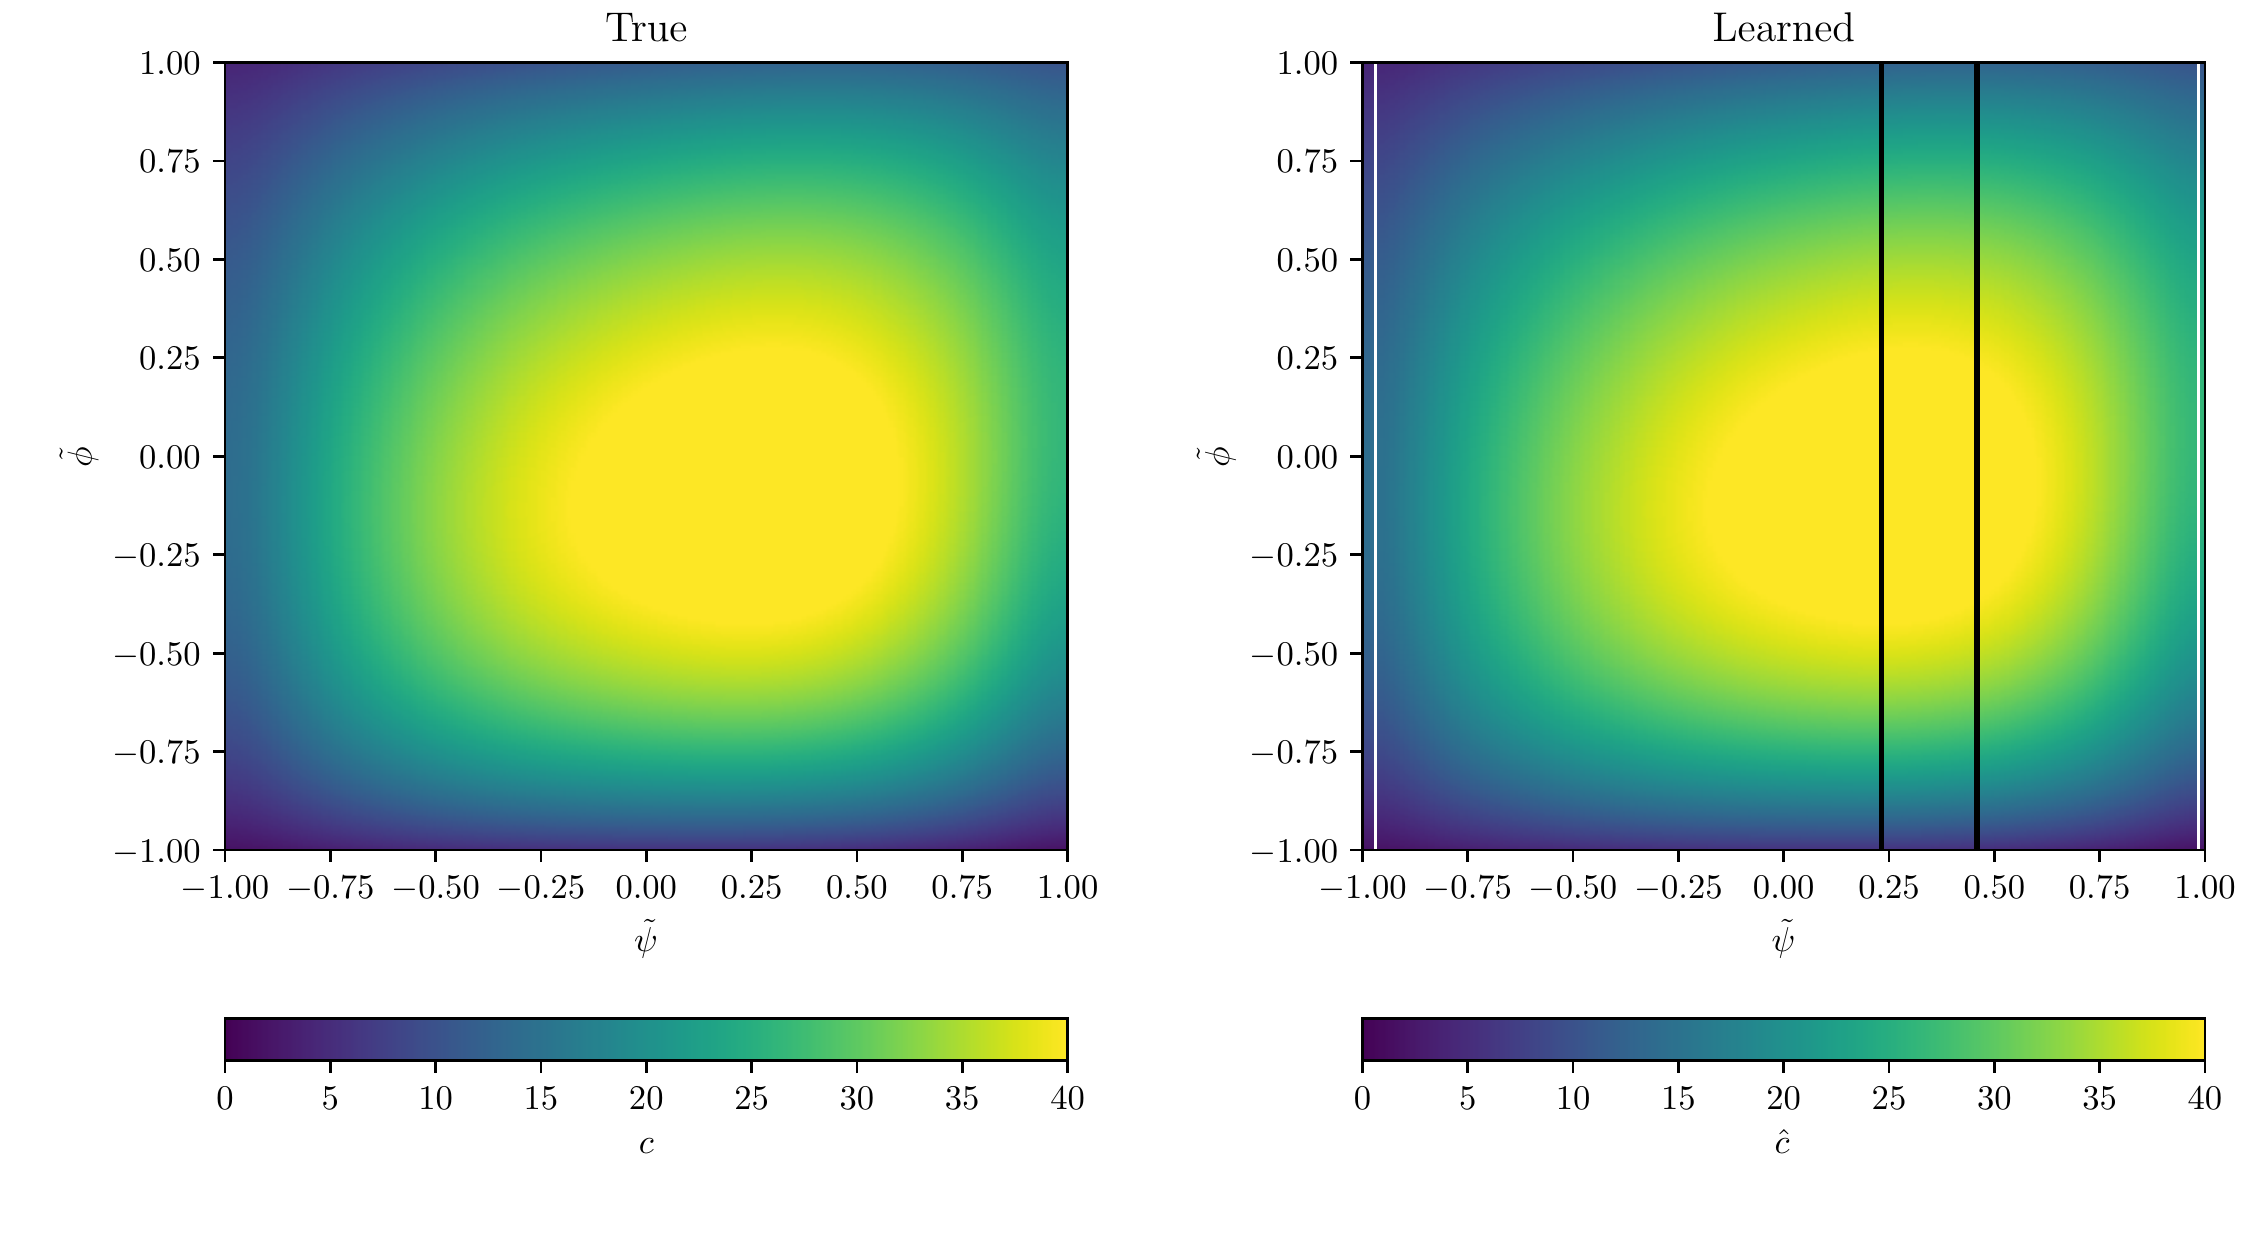}
    \caption{Left: True data as shown in Fig.~\ref{fig:learn_time}(right). Right: Data obtained by integrating the initial snapshot of the data shown on the left, but using the learned model $f$. Thereby, boundaries are provided, as indicated by the white vertical lines. In addition, the corridor around the source term is provided, as indicated by the black vertical lines.}
    \label{fig:learn_results_emergent_space_and_time}
\end{figure*}

\begin{figure*}
    \includegraphics[width=\textwidth]{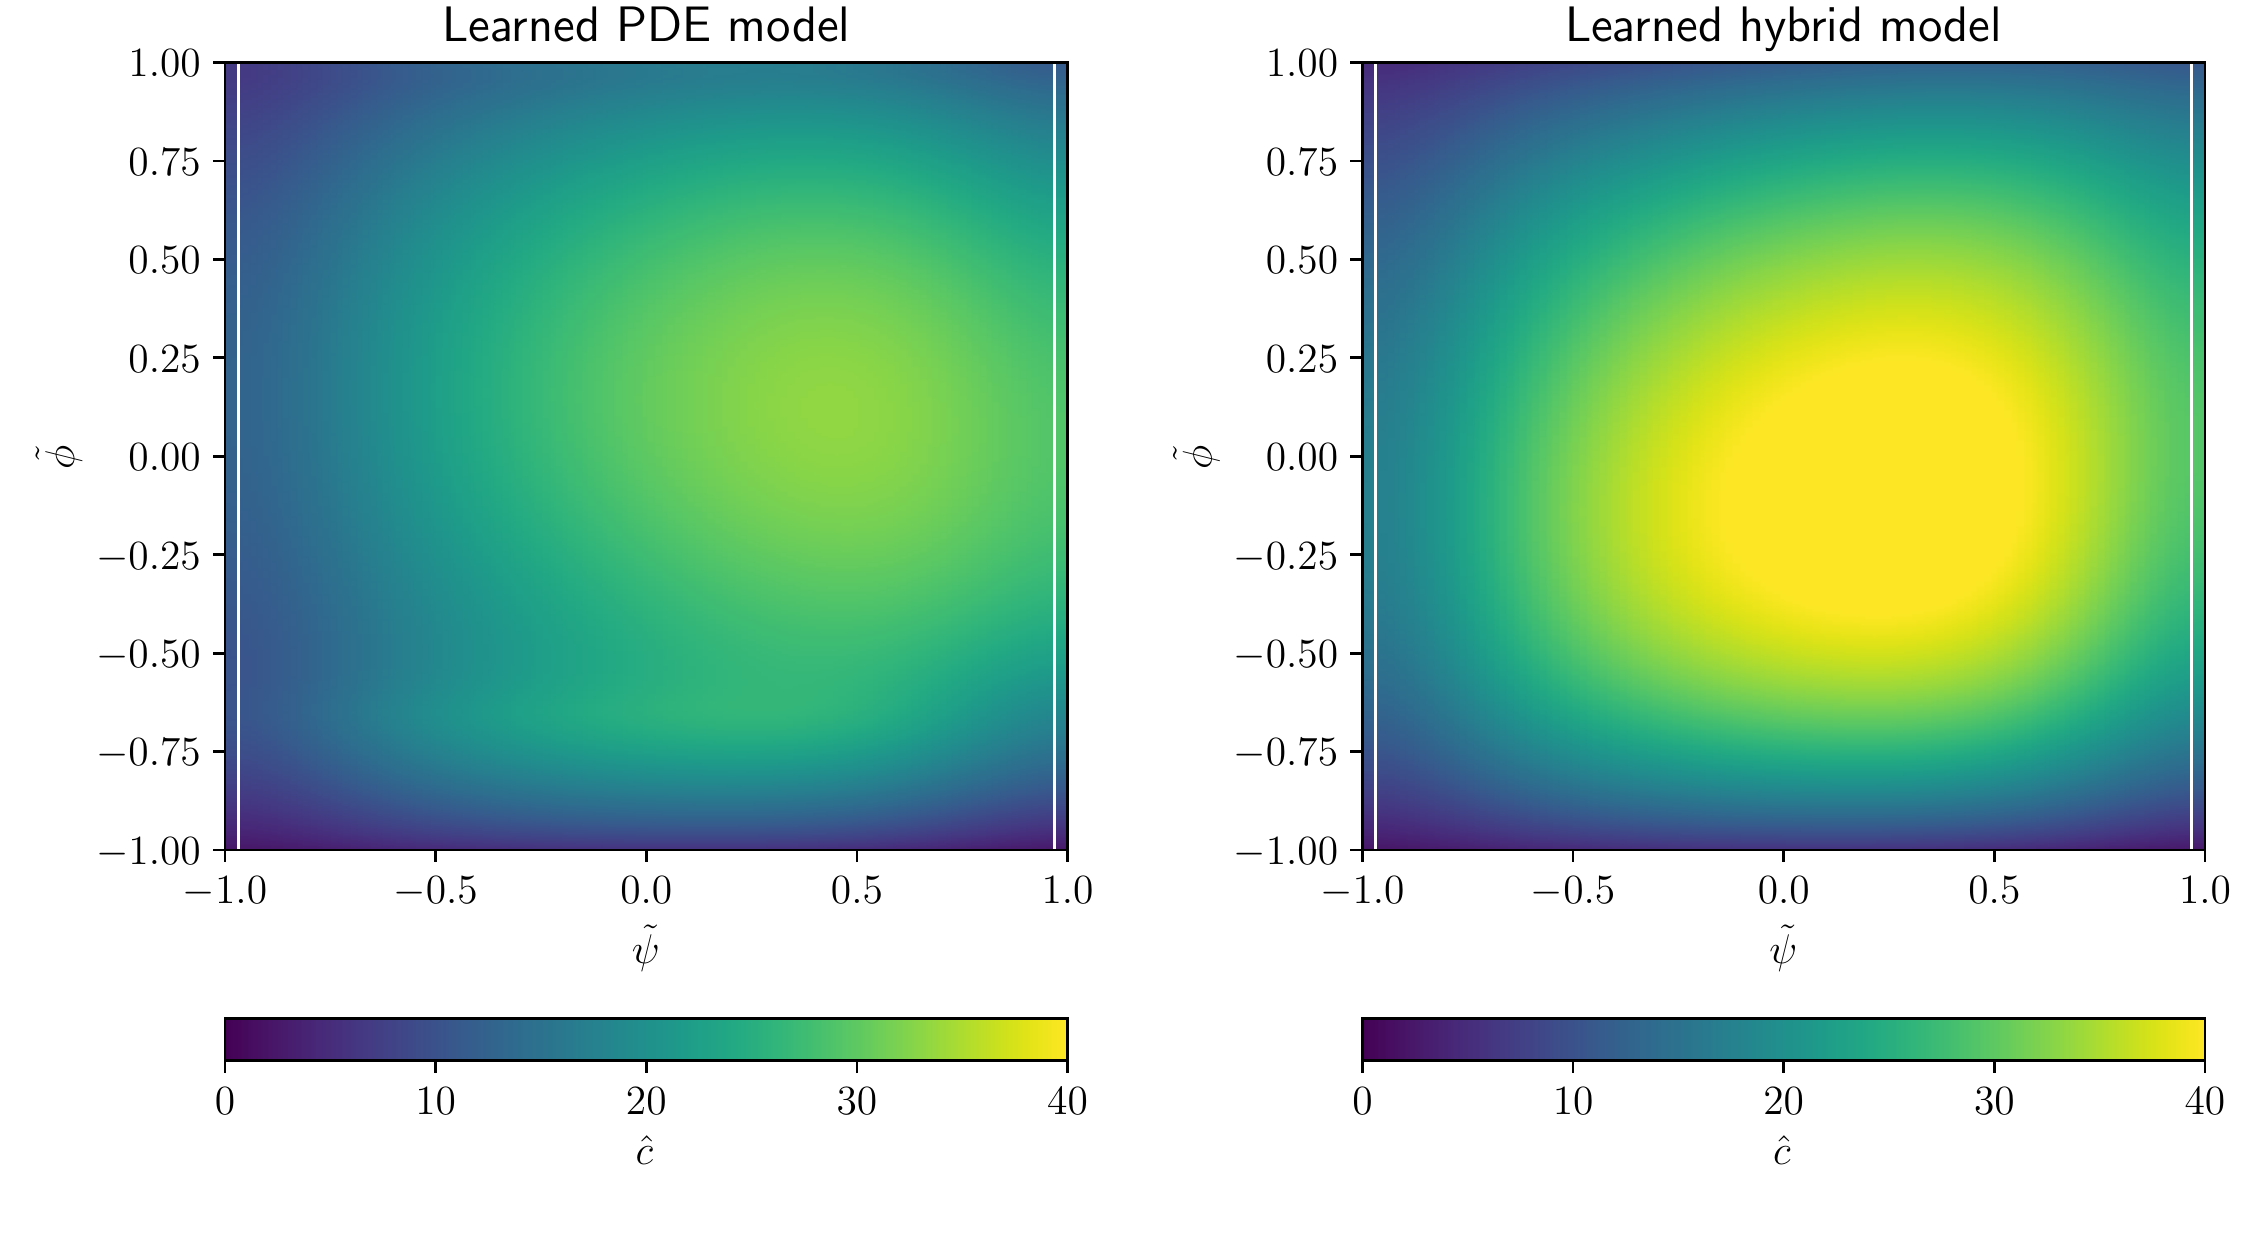}
    \caption{Left: Integration using the autonomous partial differential equation $f$ over the whole domain, using the same initial snapshot as in Fig.~\ref{fig:learn_results_emergent_space_and_time}, but without providing the source term.
    Right: Integration results using the non-autonomous hybrid model, Eq.~\eqref{eq:f_w_source}, using the same initial snapshot as in Fig.~\ref{fig:learn_results_emergent_space_and_time}. Note the visual agreement with the true data,
    as in Fig.~\ref{fig:learn_results_emergent_space_and_time}.}
    \label{fig:results_hybrid}
\end{figure*}
